# Supplementary material for: Differentially Private Federated Learning without Noise Addition: When is it Possible?
Source: arXiv:2405.04551 source file (2024-10-24)
Supplement: Supplementary file 1 [file appendix.tex]

\appendix
\section{Proof for Corollary 1}
\label{sec:proof_coro1}
\noindent\textbf{Corollary 1.} \textit{(IID users with non-singlular covariance matrix) 
Under Assumption \ref{assum0}, \ref{assum1}, \ref{assum2}, we further assume that all non-sensitive users’ local datasets are randomly sampled IID from a common distribution, which implies that the gradient updates of all users come from the identical distribution with the same mean $\mu^{(t)}$ and covariance matrix $\Sigma^{(t)}$ (i.e., $\forall j\in\mathbb{U}_{ns}, x_j^{(t)}\sim \mathcal{N}(\mu^{(t)}, \Sigma^{(t)})$}). Let $\lambda_{0,min}^{(t)}$ be the smallest eigenvalue of $\Sigma^{(t)}$. Then, the aggregated gradient from other users $x_{ns}^{(t)}$ at step $t$ can provide $(\epsilon_i^{(t)},\delta)$-DP for sensitive user $i\in\mathbb{U}_{s}$ with $\epsilon_i^{(t)}=\frac{2C\sqrt{2\log\frac{1.25}{\delta}}}{B\sqrt{|\mathbb{U}_{ns}|\lambda_{min}^{(t)}}}$ for high privacy region ($\epsilon_i^{(t)}\in(0,1)$) and $\epsilon_i^{(t)}=\frac{2C^2}{B^2|\mathbb{U}_{ns}|\lambda_{0,min}^{(t)}}$ for high privacy region ($\epsilon_i^{(t)}\geq 1$),
where $|\mathbb{U}_{ns}|$ is the number of non-sensitive users.

\begin{proof}
    Since $\forall j\in\mathbb{U}_{ns}, x_j^{(t)}\sim \mathcal{N}(\mu^{(t)}, \Sigma^{(t)})$, we have $\Sigma_{ns}^{(t)}=\sum_{j\in\mathbb{U}_{ns}}\Sigma_{j}^{(t)}=|\mathbb{U}_{ns}|\Sigma^{(t)}$. Hence, the smallest eigenvalue of $\Sigma_{ns}^{(t)}$ will be $|\mathbb{U}_{ns}|\lambda_{0,min}^{(t)}$. Based on Eq. \ref{eq:lambda1} in Theorem \ref{theorem1}, in high privacy region where $\epsilon_i^{(t)}\in(0,1)$, we have $\epsilon_i^{(t)}=\frac{2C\sqrt{2\log\frac{1.25}{\delta}}}{B\sqrt{|\mathbb{U}_{ns}|\lambda_{0,min}^{(t)}}}$. In low privacy region where $\epsilon_i^{(t)}\geq 1$, we have $\epsilon_i^{(t)}=\frac{2C^2}{B^2|\mathbb{U}_{ns}|\lambda_{0,min}^{(t)}}$.
\end{proof}

\section{Proof for Corollary 2}
\label{sec:proof_coro2}
\noindent\textbf{Corollary 2.} \textit{(IID users with singular covariance matrix) 
Under Assumption \ref{assum1}, Assumption \ref{assum3}, we further assume that all non-sensitive users’ local datasets are randomly sampled IID from a common distribution, which implies that the gradient updates of all non-sensitive users come from the identical distribution with the same mean $\mu^{(t)}$ and covariance matrix $\Sigma^{(t)}$ (i.e., $\forall j\in\mathbb{U}_{ns}, x_j^{(t)}\sim \mathcal{N}(\mu^{(t)}, \Sigma^{(t)})$. Let $\lambda_{min}^{(t),*}$ be the smallest non-zero eigenvalue of $\Sigma^{(t)}$. Then, the aggregated gradient from all non-sensitive users $x_{ns}^{(t)}$ at step $t$ can provide $(\epsilon_i^{(t)},\delta)$-DP for sensitive user $i\in\mathbb{U}_{s}$ with $\epsilon_i^{(t)}=\frac{2C\sqrt{2\log\frac{1.25}{\delta}}}{B\sqrt{|\mathbb{U}_{ns}|\lambda_{min}^{(t),*}}}$ for high privacy region ($\epsilon_i^{(t)}\in(0,1)$) and $\epsilon_i^{(t)}=\frac{2C^2}{B^2|\mathbb{U}_{ns}|\lambda_{0,min}^{(t),*}}$ for high privacy region ($\epsilon_i^{(t)}\geq 1$),
where $|\mathbb{U}_{ns}|$ is the number of non-sensitive users.
}
\begin{proof}
    Since $\forall j\in\mathbb{U}_{ns}, x_j^{(t)}\sim \mathcal{N}(\mu^{(t)}, \Sigma^{(t)})$, we have $\Sigma_{ns}^{(t)}=\sum_{j\in\mathbb{U}_{ns}}\Sigma_{j}^{(t)}=|\mathbb{U}_{ns}|\Sigma^{(t)}$. Hence, the smallest non-zero eigenvalue of $\Sigma_{ns}^{(t)}$ will be $|\mathbb{U}_{ns}|\lambda_{0,min}^{(t),*}$. By applying Theorem \ref{theorem2}, Corollary \ref{coro2} holds.
\end{proof}

\section{Proof for Theorem 3}
\label{sec:proof_theorem3}
\noindent\textbf{Theorem 3.} \textit{
Under Assumption \ref{assum0},\ref{assum1} and Assumption \ref{assum5},\ref{assum6}, the aggregated gradient from non-sensitive users $x_{ns}^{(t)}$ at step $t$ can provide $(\epsilon_i^{(t)},\delta+\delta_c)$-DP for sensitive user $i$, where $\epsilon_i^{(t)}=p(\lambda_{min}^{(t)},\delta)$, and $\lambda_{min}^{(t)}$ is the smallest eigenvalue of $\Sigma_{ns}^{(t)}$, $\delta_c=(1+e^{\epsilon_i^{(t)}})\delta_0$.}
\begin{proof}
Assume that $x_{i,1}^{(t)}$ and $x_{i,2}^{(t)}$ are two gradient instance of $x_{i}^{(t)}$ at step $t$, which are calculated from two local datasets $D_i^{1}$ and $D_i^{2}$ differing from one data points. Then, $\forall X \subseteq Range(x_{i}^{(t)}+x_{ns}^{(t)})$ and $\forall$ $x_{i,1}^{(t)}$ and $x_{i,2}^{(t)}$,  we have:
\begin{align}
    & Pr[x_{i,1}^{(t)}+x_{ns}^{(t)}\in X] - e^{\epsilon_i^{(t)}}Pr[x_{i,2}^{(t)}+x_{ns}^{(t)}\in X]\\
    \leq & (Pr[x_{i,1}^{(t)}+n_{ns}^{(t)}\in Z] + \delta_0) - e^{\epsilon_i^{(t)}}(Pr[x_{i,2}^{(t)}+n_{ns}^{(t)}\in Z]-\delta_0)\\
    \leq & Pr[x_{i,1}^{(t)}+n_{ns}^{(t)}\in Z] - e^{\epsilon_i^{(t)}}Pr[x_{i,2}^{(t)}+n_{ns}^{(t)}\in Z] + (1+e^{\epsilon_i^{(t)}})\delta_0.
\end{align}
where $n_{ns}^{(t)}\sim N(\mu_{ns}^{(t)},\Sigma_{ns}^{(t)})$ is a Gaussian random vector. Based on Theorem \ref{theorem1}, we have:
\begin{align}
    Pr[x_{i,1}^{(t)}+n_{ns}^{(t)}\in Z] - e^{\epsilon_i^{(t)}}Pr[x_{i,2}^{(t)}+n_{ns}^{(t)}\in Z]\leq\delta.
\end{align}

Hence, we can derive:
\begin{align}
    & Pr[x_{i,1}^{(t)}+x_{ns}^{(t)}\in X] - e^{\epsilon_i^{(t)}}Pr[x_{i,2}^{(t)}+x_{ns}^{(t)}\in X]\\
    \leq & \delta + (1+e^{\epsilon_i^{(t)}})\delta_0
    = \delta + \delta_c.
\end{align}
\end{proof}

\section{Experimental Details For \texorpdfstring{$\epsilon$}{e} Calculation}
\label{sec:appendix}
\noindent\textbf{UCI Wine dataset.} For our experiments on UCI Wine dataset, each user's local dataset has around 400 data points. Hence, we set $\delta$ as $1\times 10^{-3}$. We use FedSGD for calculating the model update of each user with batch size $B=100$. For each user at training round $t$, we clip each individual gradient calculated from each data point to bound its $L_2$ norm by $C=2$. We use Gaussian gradient descent for both WF-DP and LDP, where we use all the data points to estimate the mean and covariance matrix of the model update of each user.
%it will provide an amplification effect of $q=\frac{1}{|D_i|}=\frac{1}{255}$ for $\epsilon$. 
Moreover, we observe that the minimal eigenvalues of the covariance matrix of each user's model update is around 0.05. Therefore, by selecting the number of non-sensitive users $|\mathcal{U}_{ns}|$ from $\{5,10,20,50\}$ and train the model for $T=50$ rounds, we will get $\epsilon$ (i.e. the privacy budget) from $\{9.49, 7.02, 4.96, 3.08\}$.

\noindent\textbf{MNIST \& CIFAR10 dataset.} For our experiments on MNIST and CIFAR10 dataset, each user's local dataset has less than 1000 training images. Hence, we set $\delta$ as $1e-3$. We use FedSGD for calculating the model update of each user with batch size $B=100$. For each user at training round $t$, we clip each individual gradient calculated from each data point to bound its $L_2$ norm by $C=2$. We use Gaussian gradient descent for both WF-DP and LDP, where we use all the data points to estimate the mean and covariance matrix of the model update of each user. Moreover, we train the model for $T=100$ rounds. Therefore, based on the algorithm in \cite{gopi2021numerical}, when we set $|\mathcal{U}_{ns}|=10$, $\sigma$ from $\{0.05, 0.1, 0.2\}$ will lead to $\epsilon$ (i.e. the privacy budget) from $\{9.55, 4.77, 2.39\}$; when we set $|\mathcal{U}_{ns}|=20$, $\sigma$ from $\{0.05, 0.1, 0.2\}$ will lead to $\epsilon$ (i.e. the privacy budget) from $\{6.76, 3.38, 1.69\}$; when we set $|\mathcal{U}_{ns}|=50$, $\sigma$ from $\{0.05, 0.1, 0.2\}$ will lead to $\epsilon$ (i.e. the privacy budget) from $\{4.27, 2.11, 1.06\}$.

\noindent\textbf{FEMNIST dataset.} For our experiments on FEMNIST dataset, each user's local dataset has a few hundreds of training images, hence we set $\delta$ as $1e-3$. We use FedAvg for calculating the model update of each user. At each training round, we randomly select 10 out of 100 sensitive users, it will provide an amplification effect of $q=\frac{1}{100}$ for $\epsilon$. For each user at training round $t$, we clip each individual gradient calculated from each data point to bound its $L_2$ norm by $C=1$. Note that in order to generate Gaussian model update for FedAvg, we repeat the local training process of each user for $M=100$ times to get 100 local model updates, estimate the mean and covariance matrix of these 100 model updates, and then generate Gaussian model update based on the estimated mean and covariance matrix. Moreover, we set the number of non-sensitive users $|\mathcal{U}_{ns}|=50$ and train the model for $T=100$ rounds. Therefore, based on the algorithm in \cite{gopi2021numerical}, $\sigma$ from $\{0.05, 0.1, 2\}$ will lead to $\epsilon$ (i.e. the privacy budget) from $\{72.09, 13.02, 3.33\}$. 

\noindent\textbf{Yelp Review dataset.} For our experiments on Yelp Review dataset, we make each user's local dataset contain 1000 training images, hence we set $\delta$ as $1e-3$. We use FedSGD for calculating the model update of each user with batch size 100. For each user at training round $t$, we clip each individual gradient calculated from each data point to bound its $L_2$ norm by $C=2$. We use Gaussian gradient descent for both WF-DP and LDP, where we use all the data points to estimate the mean and covariance matrix of the model update of each user. Moreover, we set the number of non-sensitive users $|\mathcal{U}_{ns}|=50$ and train the model for $T=100$ rounds. Therefore, based on the algorithm in \cite{gopi2021numerical}, $\sigma$ from $\{0.05, 0.1, 0.2\}$ will lead to $\epsilon$ (i.e. the privacy budget) from $\{4.27, 2.11, 1.06\}$.
